# Supplementary material for: Robust multi-outcome regression with correlated covariate blocks using fused LAD-lasso
Source: arXiv:2212.00461 source file (2022-12-01)
Supplement: Supplementary file 1 [file appendix.tex]

\appendix
\section{Estimation of the multi-outcome fused lasso regression coefficients}

The objective function is
\begin{eqnarray*}
\label{fused_lasso1}
v(\bo B) & = &\frac1n\sum_{i=1}^n\|\bo y_i- \bo B'\bo x_i\|^2 
+ \lambda_1\sum_{j=1}^p\gamma_j\|\bs\beta_j\|
+ \lambda_2\sum_{k=1}^{p-1}\delta_k\|\bs\beta_{k+1}-\bs\beta_{k}\|
\\
&=&
\frac1n f(\bo B) + \lambda_1 g(\bo B) +  \lambda_2 h(\bo B),
\end{eqnarray*}
where
$$
f(\bo B) = \sum_{i=1}^n\|\bo y_i- \bo B'\bo x_i\|^2,\ \ g(\bo B) = \sum_{j=1}^p\gamma_j\|\bs\beta_j\| \ \ \text{and}\ \ 
h(\bo B) = \sum_{k=1}^{p-1}\delta_k\|\bs\beta_{k+1}-\bs\beta_{k}\|.
$$
\begin{eqnarray*}
\label{fused_lasso2}
f(\bo B) & = & \sum_{i=1}^n\|\bo y_i-\bo B'\bo x_i\|^2 \\
& = &
\tr[(\bo Y-\bo X\bo B)(\bo Y-\bo X\bo B)']\\
& = &
\vecc((\bo Y-\bo X\bo B)')'
\vecc((\bo Y-\bo X\bo B)')
\\
& = &
(\bo y - (\bo X\otimes\bo I_q)\bs\beta)'
(\bo y  - (\bo X\otimes\bo I_q)\bs\beta)\\
& =&
\bo y'\bo y 
-2\bs\beta'(\bo X'\otimes\bo I_q)\bo y
+\bs\beta'(\bo X'\bo X\otimes\bo I_q)\bs\beta
\end{eqnarray*}

\begin{eqnarray*}
\label{fused_lasso2b}
\frac{\partial f(\bo B) }{\partial\bs\beta}
 & = & 
-2(\bo X'\otimes\bo I_q)\bo y
+2(\bo X'\bo X\otimes\bo I_q)\bs\beta\\
& = &
-2\vecc[(\bo X'\bo Y-\bo X'\bo X\bo B)']
\end{eqnarray*}

\begin{eqnarray*}
\label{fused_lasso2c}
\frac{\partial f(\bo B) }{\partial\bo B}
 & = & 
-2(\bo X'\bo Y-\bo X'\bo X\bo B)
\end{eqnarray*}

\begin{eqnarray*}
\label{fused_lasso3}
g(\bo B) = \sum_{j=1}^p\gamma_j\|\bs\beta_j\|
= \sum_{j=1}^p\gamma_j(\bs\beta_j'\bs\beta_j)^{1/2}
\end{eqnarray*}

\begin{eqnarray*}
\label{fused_lasso3b}
\frac{\partial g(\bo B) }{\partial\bs\beta}
=
\begin{pmatrix}
\gamma_0\bo u(\bs\beta_0)\\
\gamma_1\bo u(\bs\beta_1)\\
\vdots\\
\gamma_p\bo u(\bs\beta_p)
\end{pmatrix}
=
\begin{pmatrix}
\bo 0_q\\
\gamma_1\bo u(\bs\beta_1)\\
\vdots\\
\gamma_p\bo u(\bs\beta_p)
\end{pmatrix}
=
\vecc[\bo U(\bo B)'\diag(\bs\gamma)]
\end{eqnarray*}
where
$$
\bo u(\bs\beta_j)
=
\begin{cases}
\bo 0, & \text{if $\|\bs\beta_j\|=0$,}\\
\|\bs\beta_j\|^{-1}\bs\beta_j,
& \text{if $\|\bs\beta_j\|\neq0$}
\end{cases}
$$
is the spatial sign of $\bs\beta_j$,
$$
\bo U(\bo B)
=
\begin{pmatrix}
\bo u(\bs\beta_0)' \\ 
\bo u(\bs\beta_1)' \\
\vdots\\ 
\bo u(\bs\beta_p)'
\end{pmatrix}
$$
and
$$
\diag(\bs\gamma)
=
\begin{pmatrix}
0 & 0        & \cdots & 0\\
0 & \gamma_1 & \cdots & 0\\
\vdots & \vdots & \ddots & \vdots\\
0 & 0   & \cdots & \gamma_p
\end{pmatrix}.
$$

\begin{eqnarray*}
\label{fused_lasso3c}
\frac{\partial g(\bo B) }{\partial\bo B}
=
\diag(\bs\gamma)\bo U(\bo B)
\end{eqnarray*}

\begin{eqnarray*}
\label{fused_lasso4}
h(\bo B) = \sum_{k=1}^{p-1}\delta_k\|\bs\beta_{k+1}-\bs\beta_{k}\| = 
\sum_{k=1}^{p-1}\delta_k
[
(\bs\beta_{k+1}-\bs\beta_{k})'
(\bs\beta_{k+1}-\bs\beta_{k})
]^{1/2}
\end{eqnarray*}

\begin{eqnarray*}
\label{fused_lasso5}
\frac{\partial}{\partial\bs\beta_s} h(\bo B) & = & 
\frac{1}{2}\sum_{k=1}^{p-1}\delta_k
\|\bs\beta_{k+1}-\bs\beta_{k}\|^{-1}
\frac{\partial}{\partial\bs\beta_s}
(\bs\beta_{k+1}-\bs\beta_{k})'
(\bs\beta_{k+1}-\bs\beta_{k})
\\
& = &
\begin{cases}
\bo 0_q, & \text{if $s=0$,}\\
-\delta_{1}\bo u(\bs\beta_{2}-\bs\beta_{1}), & \text{if $s=1$,}\\
\delta_{s-1}\bo u(\bs\beta_s-\bs\beta_{s-1})-\delta_{s}\bo u(\bs\beta_{s+1}-\bs\beta_{s}), & \text{if $2\leq s\leq p-1$,}\\
\delta_{p-1}\bo u(\bs\beta_p-\bs\beta_{p-1}), & \text{if $s=p$.}\\
\end{cases}
\end{eqnarray*}

\begin{eqnarray*}
\label{fused_lasso6}
\frac{\partial}{\partial\bs\beta} h(\bo B) & = & 
\begin{pmatrix}
\bo 0_q \\
\bo 0_q \\
\delta_{1}\bo u(\bs\beta_2-\bs\beta_{1}) \\
\delta_{2}\bo u(\bs\beta_3-\bs\beta_{2}) \\
\vdots \\
\delta_{p-2}\bo u(\bs\beta_{p-1}-\bs\beta_{p-2}) \\
\delta_{p-1}\bo u(\bs\beta_p-\bs\beta_{p-1})
\end{pmatrix}
-
\begin{pmatrix}
\bo 0_q \\
\delta_{1}\bo u(\bs\beta_{2}-\bs\beta_{1}) \\
\delta_{2}\bo u(\bs\beta_3-\bs\beta_{2}) \\
\delta_{3}\bo u(\bs\beta_4-\bs\beta_{3}) \\
\vdots \\
\delta_{p-1}\bo u(\bs\beta_{p}-\bs\beta_{p-1}) \\
\bo 0_q
\end{pmatrix}
\end{eqnarray*}

\begin{eqnarray*}
\label{fused_lasso7}
&&\begin{pmatrix}
\bo 0_q' \\
\delta_{0}(\bs\beta_1-\bs\beta_{0})' \\
\delta_{1}(\bs\beta_2-\bs\beta_{1})' \\
\delta_{2}(\bs\beta_3-\bs\beta_{2})' \\
\vdots \\
\delta_{p-2}(\bs\beta_{p-1}-\bs\beta_{p-2})' \\
\delta_{p-1}(\bs\beta_p-\bs\beta_{p-1})'
\end{pmatrix}
-
\begin{pmatrix}
\delta_{0}(\bs\beta_1-\bs\beta_{0})' \\
\delta_{1}(\bs\beta_{2}-\bs\beta_{1})' \\
\delta_{2}(\bs\beta_3-\bs\beta_{2})' \\
\delta_{3}(\bs\beta_4-\bs\beta_{3})' \\
\vdots \\
\delta_{p-1}(\bs\beta_{p}-\bs\beta_{p-1})' \\
\bo 0_q'
\end{pmatrix}
\\
&&=
\begin{pmatrix}
\bo 0_{q}'\\
\bo D\bo W\bo B
\end{pmatrix}
-
\begin{pmatrix}
\bo D\bo W\bo B\\
\bo 0_{q}'
\end{pmatrix}
=
\bo A\bo W\bo B,
\end{eqnarray*}
where
$$
\bo A =
\begin{pmatrix}
\bo 0_{p}'\\
\bo D
\end{pmatrix}
-
\begin{pmatrix}
\bo D\\
\bo 0_{p}'
\end{pmatrix},
$$
\begin{eqnarray*}
\bo W  & = & 
\begin{pmatrix}
\bo 0_{p} & \bo I_{p}
\end{pmatrix}
-
\begin{pmatrix}
\bo I_{p} &  \bo 0_{p}
\end{pmatrix} \\
& = &
\begin{pmatrix}
-1   & ~~1        & 0        & 0      & \cdots & ~~0 & 0\\
~~0 & ~~0         & -1       & 1      & \cdots & ~~0 & 0\\
\vdots & ~~\vdots & ~~\vdots & \vdots & \ddots & ~~1 & 0\\
~~0 & ~~0         & ~~0      & 0      & \cdots &  -1 & 1 
\end{pmatrix},
\end{eqnarray*}
and
$$
\bo D = \diag(\bs\delta) = \diag(0,\delta_1,\cdots,\delta_{p-1}) =
\begin{pmatrix}
0      & 0        & 0        & \cdots & 0\\
0      & \delta_1 & 0        & \cdots & 0\\
0      & 0        & \delta_2 & \cdots & 0\\
\vdots & \vdots   & \vdots   & \ddots & \vdots \\
0      & 0        & 0        & \cdots & \delta_{p-1}\\
\end{pmatrix}
$$

$$
\frac{\partial}{\partial\bs\beta} h(\bo B) =
\vecc[(\bo A\ \bo U(\bo W\bo B))'] = \vecc[\bo U(\bo W\bo B)'\bo A']
$$

$$
\frac{\partial}{\partial\bo B} h(\bo B) =
\bo A\ \bo U(\bo W\bo B)
$$

$$
\frac{\partial}{\partial\bs\beta} v(\bo B) =
-\frac{2}{n}\vecc[(\bo X'\bo Y-\bo X'\bo X\bo B)']
+\lambda_1\vecc[\bo U(\bo B)'\diag(\bs\gamma)]
+\lambda_2\vecc[\bo U(\bo W\bo B)'\bo A']
$$

$$
\frac{\partial}{\partial\bo B} v(\bo B) =
-\frac{2}{n}(\bo X'\bo Y-\bo X'\bo X\bo B)
+\lambda_1\diag(\bs\gamma)\bo U(\bo B)
+\lambda_2\bo A\bo U(\bo W\bo B)
$$

\section{Estimation of the multi-outcome LAD regression coefficients}

The objective function is
\begin{eqnarray*}
\label{LAD-regression}
w(\bo B) & = &\sum_{i=1}^n\|\bo y_i- \bo B'\bo x_i\|
= \sum_{i=1}^n[(\bo y_i- \bo B'\bo x_i)'(\bo y_i- \bo B'\bo x_i)]^{1/2}
\\
& = &
\sum_{i=1}^n
[
\bo y_i'\bo y_i-\bo y_i'\bo B'\bo x_i
-\bo x_i'\bo B\bo y_i+\bo x_i'\bo B\bo B'\bo x_i
]^{1/2}
\end{eqnarray*}

\begin{eqnarray*}
\label{LAD-regression2}
\frac{\partial w(\bo B)}{\partial \bo B}
 & = &
\frac{1}{2}\sum_{i=1}^n\|\bo y_i- \bo B'\bo x_i\|^{-1}
[-2\bo x_i\bo y_i'+2\bo x_i\bo x_i'\bo B]
\\
& = &
-\sum_{i=1}^n\|\bo y_i- \bo B'\bo x_i\|^{-1}
\bo x_i(\bo y_i-\bo B'\bo x_i)'
\\
& = &
-\sum_{i=1}^n\bo x_i\bo u(\bo y_i-\bo B'\bo x_i)'
=
-\bo X'\bo U
\end{eqnarray*}

\begin{eqnarray*}
\label{LAD-regression3}
\frac{\partial w(\bo B)}{\partial\bs\beta}
 & = &
 \vecc\left(\frac{\partial w(\bo B)}{\bo B'}\right)
 =
 -\vecc(\bo U'\bo X)
=
 -(\bo X'\otimes\bo I_q)\vecc(\bo U')
 \end{eqnarray*}

\begin{eqnarray*}
\label{LAD-regression4}
\frac{\partial^2 w(\bo B)}{\partial\bs\beta\partial\bs\beta'}
 & = &
  \frac{\partial}{\partial\bs\beta}
  \left[
  \frac{\partial w(\bo B)}{\partial\bs\beta'}
  \right] 
 = 
 -\frac{\partial}{\partial\bs\beta}
 \vecc(\bo U')'
  (\bo X\otimes\bo I_q)
\end{eqnarray*}

\begin{eqnarray*}
\label{LAD-regression5}
 &&\frac{\partial}{\partial\bs\beta}\bo u(\bo y_i-\bo B'\bo x_i)'
=
\frac{\partial}{\partial\bs\beta}
\|\bo y_i- \bo B'\bo x_i\|^{-1}
(\bo y_i-\bo B'\bo x_i)'\\
&&=
\left[
\frac{\partial}{\partial\bs\beta}
\|\bo y_i- \bo B'\bo x_i\|^{-1}
\right] 
(\bo y_i-\bo B'\bo x_i)'
+
\|\bo y_i- \bo B'\bo x_i\|^{-1}
\frac{\partial}{\partial\bs\beta}
(\bo y_i-\bo B'\bo x_i)'
\end{eqnarray*}

\begin{eqnarray*}
\label{LAD-regression6}
&&\frac{\partial}{\partial\bo B'}
\|\bo y_i- \bo B'\bo x_i\|^{-1}
=
-\frac{1}2\|\bo y_i- \bo B'\bo x_i\|^{-3}
\frac{\partial}{\partial\bo B'}
(\bo y_i'\bo y_i-2\bo y_i'\bo B'\bo x_i
+\bo x_i'\bo B\bo B'\bo x_i)
\\
&&=
-\frac{1}2\|\bo y_i- \bo B'\bo x_i\|^{-3}
(
-2\bo y_i\bo x_i'+2\bo B'\bo x_i\bo x_i'
)
=
\|\bo y_i- \bo B'\bo x_i\|^{-3}
(
\bo y_i-\bo B'\bo x_i
)\bo x_i'
\\
&&=
\|\bo y_i- \bo B'\bo x_i\|^{-2}
\bo u(\bo y_i-\bo B'\bo x_i)\bo x_i'
\end{eqnarray*}

\begin{eqnarray*}
\label{LAD-regression7}
&&\frac{\partial}{\partial\bs\beta}
\|\bo y_i- \bo B'\bo x_i\|^{-1}
=
\vecc\left(\frac{\partial}{\partial\bo B'}
\|\bo y_i- \bo B'\bo x_i\|^{-1}\right)
\\
&&=
\|\bo y_i- \bo B'\bo x_i\|^{-2}
(\bo x_i\otimes\bo I_q)
\bo u(\bo y_i-\bo B'\bo x_i)
\end{eqnarray*}

\begin{eqnarray*}
\label{LAD-regression8}
\frac{\partial}{\partial\bs\beta}
(\bo y_i-\bo B'\bo x_i)'
=
\frac{\partial}{\partial\bs\beta}
(\bo y_i'-\bo x_i'\bo B)
=
- (\bo x_i \otimes \bo I_q)
\end{eqnarray*}

\begin{eqnarray*}
\label{LAD-regression9}
 &&\frac{\partial}{\partial\bs\beta}\bo u(\bo y_i-\bo B'\bo x_i)'
\\
&=&
\left[
\frac{\partial}{\partial\bs\beta}
\|\bo y_i- \bo B'\bo x_i\|^{-1}
\right] 
(\bo y_i-\bo B'\bo x_i)'
+
\|\bo y_i- \bo B'\bo x_i\|^{-1}
\frac{\partial}{\partial\bs\beta}
(\bo y_i-\bo B'\bo x_i)'
\\
&=&
\|\bo y_i- \bo B'\bo x_i\|^{-1}
(\bo x_i\otimes\bo I_q)
\bo u(\bo y_i-\bo B'\bo x_i)
\bo u(\bo y_i-\bo B'\bo x_i)'
\\
&&-
\|\bo y_i- \bo B'\bo x_i\|^{-1}
(\bo x_i \otimes \bo I_q)
\\
& = &
\|\bo y_i- \bo B'\bo x_i\|^{-1}
(\bo x_i\otimes\bo I)
[
\bo u(\bo y_i-\bo B'\bo x_i)
\bo u(\bo y_i-\bo B'\bo x_i)'
-\bo I_q
]
\end{eqnarray*}

\begin{eqnarray*}
\label{LAD-regression10}
\frac{\partial^2 w(\bo B)}{\partial\bs\beta\partial\bs\beta'}
 & = &
 -\sum_{i=1}^n
 \left[ 
  \frac{\partial}{\partial\bs\beta}\bo u(\bo y_i-\bo B'\bo x_i)'
  \right] 
  (\bo x_i'\otimes\bo I_q)
  \\
  & = &
  -\sum_{i=1}^n
  \|\bo y_i- \bo B'\bo x_i\|^{-1}
  (\bo x_i \otimes \bo I_q)
[
\bo u(\bo y_i-\bo B'\bo x_i)
\bo u(\bo y_i-\bo B'\bo x_i)'
-\bo I_q
]
(\bo x_i'\otimes\bo I_q)
\\
& = &
  -\sum_{i=1}^n
  \|\bo y_i- \bo B'\bo x_i\|^{-1}
  (\bo x_i \otimes \bo I_q)
[
\bo u_i
\bo u_i'
-\bo I_q
]
(\bo x_i'\otimes\bo I_q)
\\
& = &
  -\sum_{i=1}^n
  \|\bo y_i- \bo B'\bo x_i\|^{-1}
(\bo x_i\bo x_i')\otimes
(
\bo u_i
\bo u_i'
-\bo I_q
)
\end{eqnarray*}
